# Supplementary material for: Differential Private Knowledge Transfer for Privacy-Preserving Cross-Domain Recommendation
Source: arXiv:2202.04893 source file (2022-02-10)
Supplement: Supplementary file 1 [file appendix.tex]

\section{Proof of Lemma~\ref{lem:interlace_1}}

\begin{lemma} 
[Eigenvalue Interlacing for Minors] Let $\mathbf{A}$ be an $n \times n$ symmetric matrix with eigenvalues 
$\lambda_1 \leq \lambda_2 \leq \cdots \lambda_n$, and $\mathbf{B}$ be any $(n-1) \times (n-1)$ principal minor sub-matrix of $\mathbf{A}$, with eigenvalues $\mu_1 \leq \mu_2 \leq \cdots \leq \mu_{n-1}.$ Then 
$$
\lambda_i \leq \mu_i \leq \lambda_{i+1}, \quad \forall 1 \leq i \leq n-1. 
$$
\label{lem:interlace_1}
\end{lemma}

\begin{proof}
Suppose $\{ x_1, \cdots, x_n \}$ be eigenvectors of $A$ and $\{ y_1, \cdots, y_{n-1} \}$ be eigenvectors of $B$. 
Denote subspaces $V_k = \spanby \{ x_k, \cdots, x_n \}$,  $W_k = \spanby \{ y_1, \cdots, y_k \}$, and $\bar{W}_k = 
\{ \begin{bmatrix} w \\ 0 \end{bmatrix} | w \in W_k \}.$
Since $\dim(V_{k}) = n - k +1$ and $\dim(\bar{W}_k) = \dim (W_k) = k,$ the intersection of $V_k$ and $\bar{W}_k$ has a non-trivial element , i.e., there exists $\bar{w} = \begin{bmatrix} w  \\ 0 \end{bmatrix} \neq 0 $ such that 
$\bar{w}^{\intercal} A \bar{w} = w^{\intercal} B w. $
By the Min-max Theorem~\cite{Wikipedia-contributors:2021tj}, 
$$
\lambda_k = \min_{x \in V_k} \frac{x^{\intercal} A x}{x^{\intercal} x} 
\leq \frac{\bar{w}^{\intercal} A \bar{w}}{\bar{w}^{\intercal} \bar{w}} 
= \frac{w^{\intercal} B w}{w^{\intercal} w} 
\leq \max_{x \in W_k} \frac{x^{\intercal} B x}{x^{\intercal} x}
= \mu_k. 
$$
To obtain the other set of inequalities, apply the same argument to the matrices $-A$ and $-B$, which have the eigenvalues 
$-\lambda_1 \leq \cdots \leq - \lambda_n$ and $- \mu_1 \leq \cdots - \mu_{n-1}$, respectively. 
\end{proof}

\subsection{Proof of Lemma~\ref{lem:interlace_2}}

\begin{proof}
Observe that $L_{G'} = L_G + (1- \frac{w}{n}) L_{a,b}
 = L_G + (1 - \frac{w}{n}) E_{a,b}^{\intercal} E_{a,b}.$\\
Denote $ L_{G} = E_G^{\intercal} E_G, X = \begin{bmatrix} E_G & \sqrt{1-\frac{w}{n}} E_{a,b} \end{bmatrix}.$ 
and $Y = \begin{bmatrix} E_G^{\intercal} \\ \sqrt{1 - \frac{w}{n}} E_{a,b}^{\intercal} \end{bmatrix}. $
Then 
$$
YX = L_{G'} \quad \text{and} \quad XY = \begin{bmatrix} L_G & \sqrt{1 - \frac{w}{n}} E_G^{\intercal} E_{a,b} \\
\sqrt{1 - \frac{w}{n}} E_{a,b}^{\intercal} E_G & (1 - \frac{w}{n}) L_{a,b} 
\end{bmatrix}. 
$$
Thus $L_G$ is a minor of $XY$. By Lemma~\ref{lem:interlace_1}, we have the eigenvalues of $L_G$ and $XY$ interlacing. 
Furthermore, non-zero eigenvalues of $XY$ and $YX$ are the same. 
$YX = L_{G'}.$
Since all matrices are PSD, we have the eigenvalues of $L_{G'}$ interlace with those of $L_G$. 
\end{proof}

\subsection{Proof of Lemma~\ref{lem:lower}}

\begin{proof}
By the interlacing results in Lemma~\ref{lem:interlace_2}, we have 
\begin{align*}
\sigma-1 & \leq \lambda_i, \forall i; \\
\prod_{i=1}^{n-1} \sigma_i & \leq \prod_{i=1}^{n-1} \lambda_i; \\
\left( \tilde{\det}{L}_G \right)^{-1/2} &\geq \left( \tilde{\det}{L}_{G'} \right)^{-1/2}. 
\end{align*}
We want to show with probability $> 1 - \delta_0$, we have 
$$
\frac{\pdf_{E^{\intercal}_G Y} (x)}{ \pdf_{E^{\intercal}_{G'} Y} (x)} \geq \left( -\frac{1}{2} x^{\intercal} \left( L_G^{\dagger} - L_{G'}^{\dagger} \right) x \right) \geq \exp(-\epsilon_0), 
$$
i.e., with probability $> 1 - \delta_0$, 
$$
x^{\intercal} \left( L_G^{\dagger} - L_{G'}^{\dagger} \right) x \leq 2 \epsilon_0. 
$$
Since 
\begin{align*}
x^{\intercal} L_G^{\dagger} x & = x^{\intercal} L_{G}^{\dagger} L_{G'} L_{G'}^{\dagger} x \\
& = x^{\intercal} L_G^{\dagger} \left( L_G + (1 - \frac{w}{n}) x^{\intercal} L_G^{\dagger} L_{a,b} L_{G'}^{\dagger} x \right) \\
& = x^{\intercal} L_{G'}^{\dagger} x + \left( 1 - \frac{w}{n} \right) x^{\intercal} L_G^{\dagger} L_{a,b} L_{G'}^{\dagger} x \\
& = x^{\intercal} L_{G'}^{\dagger} x + \left( 1 - \frac{w}{n} \right) x^{\intercal} L_G^{\dagger} e_{a,b} e_{a,b}^{\intercal} L_{G'}^{\intercal} x,
\end{align*}
we only need to show for 
$
S = \{ x^{\intercal} L_G^{\dagger} e_{a,b} \cdot e_{a,b}^{\intercal} L_{G'}^{\dagger} x > \frac{2}{1 - \frac{w}{n}} \epsilon_0 \} ,
$
$Pr (S) < \delta_0.$

Let $v_1 = E_G L_G^{\dagger} e_{a,b}$, $v_2 = E_G L_{G'}^{\dagger} e_{a,b}$, 
then
$$w_1 =x^{\intercal} L_G^{\dagger} e_{a,b} = y^{\intercal} E_G   L_G^{\dagger} e_{a,b} = y^{\intercal} v_1 ,$$
$$w_2 =x^{\intercal} L_{G'}^{\dagger} e_{a,b} = y^{\intercal} E_G   L_{G'}^{\dagger} e_{a,b} = y^{\intercal} v_2 , $$
with 
$y \sim \GN(0, I_{n \times 1}). $

For $v_1$ and $v_2$, we have 
\begin{align*}
\| v_1 \| &= \| E_G L_G^{\dagger} e_{a,b} \| = \| V \Sigma U^{\intercal} U \Sigma^{-2} U^{\intercal} e_{a,b} \| \\
& = \| V \Sigma^{-1} U^{\intercal} e_{a,b} \| \\
& \leq \| V \| \| \Sigma^{-1} \| \| U \| \| e_{a,b} \| \\
& \leq 1 \cdot \sigma_{n-1}^{-1} \cdot 1 \cdot \sqrt{2} \\
& \leq \sqrt{2/w},
\end{align*}
\begin{align*}
\| v_2 \| &= \| E_G L_G^{\intercal} e_{a,b} \| \\
& = \| \left( E_{G'} - (1 - \frac{w}{n}) E_{a,b} \right) L_{G'}^{\dagger} e_{a,b} \| \\
& < \| E_{G'} L_{G'}^{\dagger} e_{a,b} \| + \| E_{a,b} L_{G'}^{\dagger} e_{a,b} \| \\
& \leq \frac{\sqrt{2}}{\sqrt{w}} + \frac{2}{w} \leq \frac{2}{\sqrt{w}}.
\end{align*}
\ccc{Since?} $w_1, w_2$ are linear combination of normal random variables. Thus 
$\| w_1 \| \sim \GN(0, \|v_1 \|^2 )$ and $\| w_2 \| \sim \GN(0, \| v_2 \|^2). $

By tail bound of normal distribution, we have 
$$
P( \| w_1 \| \geq \sqrt{\log(2/\delta_0)} \| v_1 \| ) \leq \exp \left( - \frac{\| v_1 \|^2 \log(2/\delta_0)}{\| v_1 \|^2} \right) < \frac{\delta_0}{2} ..
$$
Thus, with probability $> 1- \delta_0,$
$$
\| w_1 \| < \sqrt{\log(1/\delta_0)} \sqrt{\frac{2}{w}}.
$$
Similarly, we have 
$$
\| w_2 \| < \sqrt{\log(1/\delta_0)} \sqrt{\frac{4}{w}}. 
$$
Thus with probability $> 1- \delta_0,$
$$
\|w -1 w_2 \| \leq \sqrt{8} \log(2/\delta_0)/w.
$$
Combining with the definition of $w$ in Algorithm~\ref{alg:dp_graph}, we thus have that with probability $> 1- \delta_0,$
$$
\|w_1 w_2 \| \leq \frac{2}{1 - \frac{w}{n}} \epsilon_0. 
$$

\end{proof}

\subsection{Proof of Lemma~\ref{lem:upper}}

\begin{proof}
We focus the vector that is not in kernel space $x \in \mathcal{V} = \mathbf{1}^{\intercal}$. 
By the property of multivariate Gaussian distribution, we have the PDF function of $E^{\intercal}_G Y$ and $E^{\intercal}_{G'}Y$ as
\begin{eqnarray*}
 \pdf_{E^{\intercal}_G Y} (x) &=& \left( (2 \pi)^{n-1} \tilde{\det} (L_{G}) \right)^{-1/2} \exp \left( - \frac{1}{2} x^{\intercal} L_G^{\dagger} x \right),  \\
 \pdf_{E^{\intercal}_{G'} Y} (x) &=& \left( (2 \pi)^{n-1} \tilde{\det} (L_{G'}) \right)^{-1/2} \exp \left( - \frac{1}{2} x^{\intercal} L_{G'}^{\dagger} x \right). 
\end{eqnarray*}
By Lemma~\ref{lem:interlace_2}, we have $\sigma_1 \leq \lambda_i, \forall i.$  Then for every $x$ it holds that 
$$
x^{\intercal} L_{G'}^{\dagger} x \leq x^{\intercal} L_G^{\dagger} x.
$$
This induces 
$$
\exp \left( - \frac{1}{2} x^{\intercal} L_G^{\dagger} x \right) \leq \exp \left( - \frac{1}{2} x^{\intercal} L_{G'}^{\dagger} x \right).
$$
Thus,
\begin{align*}
 \frac{\pdf_{E_G^{\intercal} Y} (x)}{\pdf_{E_{G'}^{\intercal} Y (x)}}  
\leq \left( \frac{\tilde{\det} (L_{G'})}{\tilde{\det} (L_G)} \right)^{1/2}  
& = \left( \prod_{i=1}^{n-1} \frac{\lambda_i^2}{\sigma_i^2} \right)^{1/2} \\
&= \left( \prod_{i=1}^{n-1} 1 + \frac{\lambda_i^2 - \sigma_i^2}{\sigma_i^2} \right)^{1/2}  \\
&\leq \prod_{i=1}^{n-1} \exp \left( \frac{1}{2} \left( \frac{\lambda_i^2 - \sigma_i^2}{\sigma_i^2} \right) \right)  \\
&\leq \exp \left( \frac{1}{2w} \sum_{i=1}^{n-1} \left( \lambda_i^2 - \sigma_i^2 \right) \right) \\
&\leq \exp (\frac{1}{w}) \\
&\leq \exp(\epsilon_0),
\end{align*}
with the property that $\sum_{i=1}^{n-1} (\lambda_i^2 - \sigma_i^2) \leq 2$ and $\sigma_i^2 \geq  w > \epsilon_0^{-1}$.
\end{proof}
